# Supplementary material for: Dense Passage Retrieval in Conversational Search
Source: arXiv:2503.17507 source file (2025-03-21)
Supplement: Supplementary file 1 [file appendix.tex]

\newpage
\appendix
\section{Appendix}

\subsection{More Implementation Details}

\subsection{Ablation Studies}
\cx{Moving to appendix I guess}
\ja{Do we track time-to-train or cost of inference in any benchmarking exercise ? \cx{we should}}

\lx{Do we need to have the same number of metric measured for ablation study? Can we just use Dev   MRR + Trec NDCG retrieval?}

\lx{Some observation, such as learning curve stability, has to be shown with graph, not table}

\input{Tables/ablation_pass}
\input{Tables/ablation_doc}

\cx{Experiments that validate our design choices: (maybe only need the passage ranking task)
\begin{enumerate}
    \item Influence of number top K to sample negatives in ANCE
    \item ANN Refresh rate (most important in this group), the effectiveness and efficiency trade-off (continue what we have in main paper)
     \item ANCE without BM25 warm up 
\end{enumerate}
}

\subsection{Additional Results on MARCO and TREC DL Track}
\cx{hole rate and recall on MARCO Doc Dev and TREC}

\subsection{Case Studies}

\input{Figures/fig_case}
\input{Tables/case_study_tbl}

\subsection{OpenQA Dense Retrieval Results}

\cx{Additional results on other tasks: 
\begin{enumerate}
    \item OpenQA results.
    \item \ao{are there any non-retrieval tasks where ANCE can apply without too much effort? or maybe even a non-NLP task? if we can show that ANCE is a generic method not just for IR/QA that might add additional value? \cx{100\% agree the impact and I think Kaiming's CV setting is a good one... But I don't think we can get it done anytime soon... It seems require much effort (and we are not CV experts)... Maybe recommendation? I like to have FAIR's OpenQA task too.}}
\end{enumerate}
}
