# Supplementary material for: Dense Passage Retrieval in Conversational Search
Source: arXiv:2503.17507 source file (2025-03-21)
Supplement: Supplementary file 2 [file appendix.tex]

\setcounter{table}{4} %

\section{Distant Supervision}
\label{sec:distant}

When training our final \model/ model using Natural Questions, we use the passages in our collection that best match the gold context as the positive passages.
As some QA datasets contain only the question and answer pairs, it is thus interesting to see when using the passages that contain the answers as positives (i.e., the distant supervision setting), whether there is a significant performance degradation.
Using the question and answer together as the query, we run Lucene-BM25 and pick the top passage that contains the answer as the positive passage.
Table~\ref{tab:qa_ir_dist_sv} shows the performance of \model/ when trained using the original setting and the distant supervision setting.

\section{Alternative Similarity Functions \& Triplet Loss}
\label{sec:alt-sim}
\label{sec:triplet}

In addition to dot product (DP) and negative log-likelihood based on softmax (NLL), we also experiment with Euclidean distance (L2) and the triplet loss.
We negate L2 similarity scores before applying softmax and change signs of question-to-positive and question-to-negative similarities when applying the triplet loss on dot product scores. 
The margin value of the triplet loss is set to 1.
Table~\ref{tab:qa_ir_sim_and_loss} summarizes the results.
All these additional experiments are conducted using the same hyper-parameters tuned for the baseline (DP, NLL).

Note that the retrieval accuracy for our ``baseline" settings reported in Table~\ref{tab:qa_ir_dist_sv} (Gold) and Table~\ref{tab:qa_ir_sim_and_loss} (DP, NLL) is slightly better than those reported in Table 3.
This is due to a better hyper-parameter setting used in these analysis experiments, which is documented in our code release.

\section{Qualitative Analysis}
\label{sec:qual_ana}

Although \model/ performs better than BM25 in general, the retrieved passages of these two retrievers actually differ qualitatively. Methods like BM25 are sensitive to highly selective keywords and phrases, but cannot capture lexical variations or semantic relationships well.  In contrast, \model/ excels at semantic representation, but might lack sufficient capacity to represent salient phrases which appear rarely.  Table~\ref{tab:retrieved-examples} illustrates this phenomenon with two examples.  In the first example, the top scoring passage from BM25 is irrelevant, even though keywords such as \textit{England} and \textit{Ireland} appear multiple times.  In comparison, \model/ is able to return the correct answer, presumably by matching \textit{``body of water"} with semantic neighbors such as \textit{sea} and \textit{channel}, even though no lexical overlap exists.
The second example is one where BM25 does better.  The salient phrase \textit{``Thoros of Myr"} is critical, and \model/ is unable to capture it.

\begin{table}[t!]
    \setlength\tabcolsep{5pt}
    \centering
    \begin{tabular}{lcccc} \toprule
         & \tf{Top-1} & \tf{Top-5} & \tf{Top-20} & \tf{Top-100}  \\ \midrule
        {Gold} & 44.9 & 66.8 & 78.1 & 85.0 \\
        {Dist. Sup.} & 43.9 & 65.3 & 77.1 & 84.4 \\
    \bottomrule
    \end{tabular}
    \caption{
    Retrieval accuracy on the development set of Natural Questions, trained on passages that match the gold context (Gold) or the top BM25 passage that contains the answer (Dist. Sup.).
    }
    \label{tab:qa_ir_dist_sv}
\end{table}

\begin{table}[t!]
    \setlength\tabcolsep{4pt}
    \centering
    \begin{tabular}{ll|cccc}
    \toprule
    \tf{Sim} & \tf{Loss} & \multicolumn{4}{c}{\tf{Retrieval Accuracy}} \\ 
    & & Top-1 & Top-5 & Top-20 & Top-100 \\ \midrule
    \multirow{2}{*}{DP} & NLL & \tf{44.9} & \tf{66.8} & \tf{78.1} & \tf{85.0} \\
    & Triplet & 41.6 & 65.0 & 77.2 & 84.5 \\
    \midrule
    \multirow{2}{*}{L2} & NLL & 43.5 & 64.7 & 76.1 & 83.1 \\
    & Triplet & 42.2 & 66.0 & \tf{78.1} & 84.9 \\ 
    \bottomrule
    \end{tabular}
     \caption{Retrieval Top-$k$ accuracy on the development set of Natural Questions using different similarity and loss functions.} 

    \label{tab:qa_ir_sim_and_loss}
\end{table}
\setlength{\tabcolsep}{6pt} %

\begin{table*}[!t]
\scriptsize
\begin{tabular}{p{3cm}|p{6cm}|p{6cm}}
\toprule
\tf{Question} & \tf{Passage received by BM25} & \tf{Passage retrieved by \model/} \\
\midrule
\multirow{2}{3cm}{What is the body of water between England and Ireland?} & Title:British Cycling  & Title: Irish Sea\\
& \ldots  \tf{England} is not recognised as a region by the UCI, and there is no English cycling team outside the Commonwealth Games. For those occasions, British Cycling selects and supports the \tf{England} team. Cycling is represented on the Isle of Man by the Isle of Man Cycling Association.  Cycling in Northern \tf{Ireland} is organised under Cycling Ulster, part of the all-Ireland governing \tf{body} Cycling \tf{Ireland}. Until 2006, a rival governing \tf{body} existed,  \ldots & \ldots Annual traffic between Great Britain and \tf{Ireland} amounts to over 12 million passengers and of traded goods. {\color{blue}\tf{The Irish Sea}} is connected to the North Atlantic at both its northern and southern ends. To the north, the connection is through the North Channel between Scotland and Northern \tf{Ireland} and the Malin Sea. The southern end is linked to the Atlantic through the St George's Channel between Ireland and Pembrokeshire, and the Celtic Sea. \ldots \\
\midrule
\multirow{2}{3cm}{Who plays Thoros of Myr in Game of Thrones?} & Title: No One (Game of Thrones) & Title:
P\r{a}l Sverre Hagen \\ & \ldots He may be "no one," but there's still enough of a person left in him to respect, and admire who this girl is and what she's become. Arya finally tells us something that we've kind of known all along, that she's not no one, she's Arya Stark of Winterfell." "No One" saw the reintroduction of Richard Dormer and {\color{blue}\tf{Paul Kaye}}, who portrayed Beric Dondarrion and \tf{Thoros} of \tf{Myr}, respectively, in the third season, \ldots &
P\r{a}l Sverre Valheim Hagen (born 6 November 1980) is a Norwegian stage and screen actor. He appeared in the Norwegian film "Max Manus" and played Thor Heyerdahl in the Oscar-nominated 2012 film "Kon-Tiki". Pål Hagen was born in Stavanger, Norway, the son of Roar Hagen, a Norwegian cartoonist who has long been associated with Norway\'s largest daily, "VG". He lived in Jåtten, a neighborhood in the city of Stavanger in south-western Norway. \ldots \\
\bottomrule
\end{tabular}
\caption{Examples of passages returned from BM25 and \model/. Correct answers are written in {\color{blue} \tf{blue}} and the content words in the question are written in bold.}
\label{tab:retrieved-examples}
\end{table*}

\section{Joint Training of Retriever and Reader}
\label{sec:joint}

We fix the passage encoder in our joint-training scheme while allowing only the question encoder to receive backpropagation signal from the combined (retriever + reader) loss function.
This allows us to leverage the HNSW-based FAISS index for efficient low-latency retrieving, without reindexing the passages during model updates.
Our loss function largely follows ORQA's approach, which uses log probabilities of positive passages selected from the retriever model, and correct spans and passages selected from the reader model.
Since the passage encoder is fixed, we could use larger amount of retrieved passages when calculating the retriever loss.
Specifically, we get top 100 passages for each question in a mini-batch and use the method similar to in-batch negative training: all retrieved passages' vectors participate in the loss calculation for \emph{all} questions in a batch. 
Our training batch size is set to 16, which effectively gives 1,600 passages per question to calculate retriever loss.
The reader still uses 24 passages per question, which are selected from the top 5 positive and top 30 negative passages (from the set of top 100 passages retrieved from the same question).
The question encoder's initial state is taken from a \model/ model previously trained on the NQ dataset.
The reader's initial state is a BERT-base model.
In terms of the end-to-end QA results, our joint-training scheme does not provide better results compared to the usual retriever/reader training pipeline, resulting in the same 39.8 exact match score on NQ dev as in our regular reader model training.
