# Supplementary material for: Dense Passage Retrieval in Conversational Search
Source: arXiv:2503.17507 source file (2025-03-21)
Supplement: Supplementary file 3 [file appendix.tex]

\newpage
\appendix
\section{Appendix}



\subsection{More Experimental Details}
\label{app:exp}

\textbf{More Details on TREC DL Benchmarks:} 
There are two tasks in the TREC DL 2019 Track: document retrieval and passage retrieval. The training and development sets are from MS MARCO, which includes passage level relevance labels for one million Bing queries~\citep{bajaj2016ms}. The document corpus was post-constructed by back-filling the body texts of the passage's URLs and their labels were inherited from its passages~\citep{craswell2020overview}. 
The testing sets are labeled by NIST accessors on the top 10 ranked results from past Track participants~\citep{craswell2020overview}.


TREC DL official metrics include NDCG@10 on test and MRR@10 on MARCO Passage Dev. MARCO Document Dev is noisy and the recall on the DL Track testing is less meaningful due to low label coverage on DR results.
There is a two-year gap between the construction of the passage training data and the back-filling of their full document content. Some original documents were no longer available. There is also a decent amount of content changes in those documents during the two-year gap, and many no longer contain the passages. 
This back-filling perhaps is the reason why many Track participants found the passage training data is more effective than the inherited document labels. Note that the TREC testing labels are not influenced as the annotators were provided the same document contents when judging.


All the TREC DL runs are trained using these training data. Their inference results on the testing queries of the document and the passage retrieval tasks were evaluated by NIST assessors in the standard TREC-style pooling technique~\citep{voorhees2000variations}. 
The pooling depth is set to 10, that is, the top 10 ranked results from all participated runs are evaluated, and these evaluated labels are released as the official TREC DL benchmarks for passage and document retrieval tasks.


\textbf{More Details on OpenQA Experiments:} 
All the DPR related experimental settings, baseline systems, and DPR Reader are based on their open source libarary\footnote{https://github.com/facebookresearch/DPR.}. The RAG-Token reader uses their open-source release in huggingface\footnote{https://huggingface.co/transformers/master/model\_doc/rag.html}. The RAG-Seq release in huggingface is not yet stable by the time we did our experiment, thus we choose the RAG-Token in our OpenQA experiment. RAG only releases the NQ models thus we use DPR reader on TriviaQA.
We feed top 20 passages from ANCE to RAG-Token on NQ and top 100 passages to DPR's BERT Reader, following the guideline in their open-source codes. 
% which was reported to be weaker than RAG-Seq.


\textbf{More Details on Baselines:}
The most representative sparse retrieval baselines in TREC DL include the standard BM25 (``bm25base'' or ``bm25base\_p''), Best TREC Sparse Retrieval (``bm25tuned\_rm3'' or ``bm25tuned\_prf\_p'') with tuned query expansion~\citep{lavrenko2017relevance}, and Best DeepCT (``dct\_tp\_bm25e2'', doc only), which uses BERT to estimate the term importance for BM25~\citep{dai2019context}. These three runs represent the standard sparse retrieval, best classical sparse retrieval, and the recent progress of using BERT to improve sparse retrieval.
We also include the standard cascade retrieval-and-reranking systems BERT Reranker (``bm25exp\_marcomb'' or ``p\_exp\_rm3\_bert''), which is the best run using standard BERT on top of query/doc expansion, from the groups with multiple top MARCO runs~\citep{nogueira2019passage, nogueira2019document}.

\textbf{BERT-Siamese Configurations:} We follow the network configurations in ~\citet{luan2020sparsedense} in all Dense Retrieval methods, which we found provides the most stable results. 
More specifically, we initialize the BERT-Siamese model with RoBERTa base~\citep{liu2019roberta} and add a $768\times768$ projection layer on top of the last layer's ``[CLS]'' token, followed by a layer norm.


\textbf{Implementation Details:}
The training often takes about 1-2 hours per ANCE epoch, which is whenever new ANCE negative is ready, it immediately replaces existing negatives in training, without waiting.
It converges in about 10 epochs, similar to other DR baselines. The optimization uses LAMB optimizer, learning rate 5e-6 for document and 1e-6 for passage retrieval, and linear warm-up and decay after 5000 steps. More detailed hyperparameter settings can be found in our code release.


\input{Tables/hole}
\subsection{Overlap with Sparse Retrieval in TREC 2019 DL Track}
\label{app:hole}


As a nature of TREC-style pooling evaluation, only those ranked in the top 10 by the 2019 TREC participating systems were labeled. As a result, documents not in the pool and thus not labeled are all considered irrelevant, even though there may be relevant ones among them. When reusing TREC style relevance labels, it is very important to keep track of the ``hole rate'' on the evaluated systems, i.e., the fraction of the top K ranked results without TREC labels (not in the pool). A larger hole rate shows that the evaluated methods are very different from those systems that participated in the Track and contributed to the pool, thus the evaluation results are not perfect. Note that the hole rate does not necessarily reflect the accuracy of the system, only the difference of it.

In TREC 2019 Deep Learning Track, all the participating systems are based on sparse retrieval.
Dense retrieval methods often differ considerably from sparse retrievals and in general will retrieve many new documents. This is confirmed in Table~\ref{tab:hole}. All DR methods have very low overlap with the official BM25 in their top 100 retrieved documents. At most, only 25\% of documents retrieved by DR are also retrieved by BM25.  This makes the hole rate quite high and the recall metric not very informative. It also suggests that DR methods might benefit more in this year's TREC 2020 Deep Learning Track if participants are contributing DR based systems.

The MS MARCO ranking labels were not constructed based on pooling the sparse retrieval results. They were from Bing~\citep{bajaj2016ms}, which uses many signals beyond term overlap. This makes the recall metric in MS MARCO more robust as it reflects how a single model can recover a complex online system.





\subsection{Impact of Asynchronous Gap}
\label{app:lap}

\input{Figures/fluct}

Fig.~\ref{fig:fluct} illustrates the behavior of asynchronous learning with different configurations.
A large learning rate or a low refreshing rate (Figure~\ref{fig:a} and~\ref{fig:b}) leads to fluctuations as the async gap of the ANN index may drive the representation learning to undesired local optima.
Refreshing as often as every 5k Batches yields a smooth convergence (Figure~\ref{fig:c}), but requires twice as many GPU allocated to the Inferencer.
A 1:1 GPUs allocation of Trainer and Inference with appropriate learning rates is adequate to minimize the impact of async gap.
% train effective representations for dense retrieval.



\subsection{Hyperparameter Studies}
\label{app:ablation}

\input{Tables/ablation_overall}

We show the results of some hyperparameter configurations in Table~\ref{tab:ablation}. The cost of training with BERT makes it difficult to conduct a lot hyperparameter exploration.
Often a failed configuration leads to divergence early in training.
We barely explore other configurations due to the time-consuming nature of working with pretrained language models. Our DR model architecture is kept consistent with recent parallel work and the learning configurations in Table~\ref{tab:ablation} are about all the explorations we did. Most of the hyperparameter choices are decided solely using the training loss curve and otherwise by the loss in the MARCO Dev set. We found the training loss, validation NDCG, and testing performance align well in our (limited) hyperparameter explorations.


\input{Tables/case_study_tbl}



\subsection{Case Studies}
\label{app:case}

In this section, we show Win/Loss case studies between ANCE and BM25. 
Among the 43 TREC 2019 DL Track evaluation queries in the document task, ANCE outperforms BM25 on 29 queries, loses on 13 queries, and ties on the rest 1 query.
The winning examples are shown in Table~\ref{tab:win_case_study} and the losing ones are in Table~\ref{tab:loss_case_study}. Their corresponding ANCE-learned (FirstP) representations are illustrated by t-SNE in Fig.~\ref{fig:t-SNE_win_case} and Fig.~\ref{fig:t-SNE_loss_case}.

In general, we found ANCE better captures the semantics in the documents and their relevance to the query. The winning cases show the intrinsic limitations of sparse retrieval. For example, BM25 exact matches the ``most popular food'' in the query ``what is the most popular food in Switzerland'' but using the document is about Mexico. The term ``Switzerland'' only appears in the related question section of the web page.

The losing cases in Table~\ref{tab:loss_case_study} are also quite interesting. Many times we found that it is not that DR fails completely and retrieves documents not related to the query's information needs at all, which was a big concern when we started research in DR. The errors ANCE made include retrieving documents that are related just not exactly relevant to the query, for example, ``yoga pose'' for ``bow in yoga''. In other cases, ANCE retrieved wrong documents due to the lack of the domain knowledge: the pretrained language model may not know ``active margin'' is a geographical terminology, not a financial one (which we did not know ourselves and took some time to figure out when conducting this case study). There are also some cases where the dense retrieved documents make sense to us but were labeled irrelevant.

The t-SNE plots in Fig.~\ref{fig:t-SNE_win_case} and Fig.~\ref{fig:t-SNE_loss_case} show many interesting patterns of the learned representation space. The ANCE winning cases often correspond to clear separations of different document groups. For losing cases the representation space is more mixed, or there is too few relevant documents which may cause the variances in model performances. There are also many different interesting patterns in the ANCE-learned representation space. 
We include the t-SNE plots for all 43 TREC DL Track queries in the supplementary material.
More future analyses of the learned patterns in the representation space may help provide more insights on dense retrieval.  




% \input{Tables/openqa_e2e}

% \input{Tables/openqa_topvals}




% \subsection{OpenQA Dense Retrieval Results}


% \cx{Additional results DPR's OpenQA setting}

% \cx{Hopefully we can also have the results on TREC-COVD! where we know ANN is very effective.}
